# Supplementary material for: Direct experimental determination of critical disorder in one-dimensional weakly disordered photonic crystals
Source: arXiv:1810.09686 source file (2018-10-23)
Supplement: Supplementary file 1 [file Supplementary_Information.pdf]

**Supplementary Information for**

# Direct experimental determination of critical disorder in one-dimensional weakly disordered photonic crystals

## I. Finite-element analysis of the periodic array

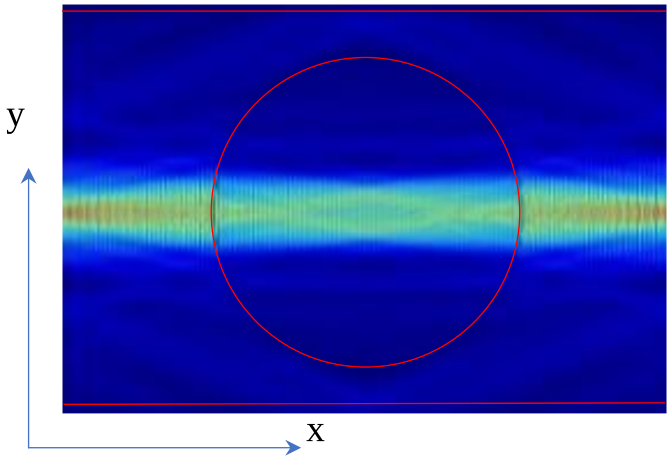


Fig. 1 Intensity distribution of the axial mode.

Finite element analysis of the fields in the single unit cell of the microresonator array was carried out using the software COMSOL MULTIPHYSICS. The technique involves computing the eigenmodes of any particular structure defined on a virtual grid. This is achieved by solving the following eigenvalue problem derived from the Maxwell's equations:$\{\nabla \times \mu^{-1} \nabla \times\}E = \epsilon \omega^2 / c^2 E$, where μ and ϵ are the relative permeability and permittivity defined at each point of the grid, which realizes the structure. The red circle in Fig.1 shows the microresonator. The eigenvalue equation is solved employing appropriate boundary conditions. Periodic boundary condition is applied in X-direction (longitudinal direction with respect to the array) and perfectly matched absorbing layers are applied in Y direction (transverse to the array) in the region beyond the red lines. Fig. 1 shows the intensity distribution of the mode of the periodic cavity array.

## II. Individual and averaged spectra

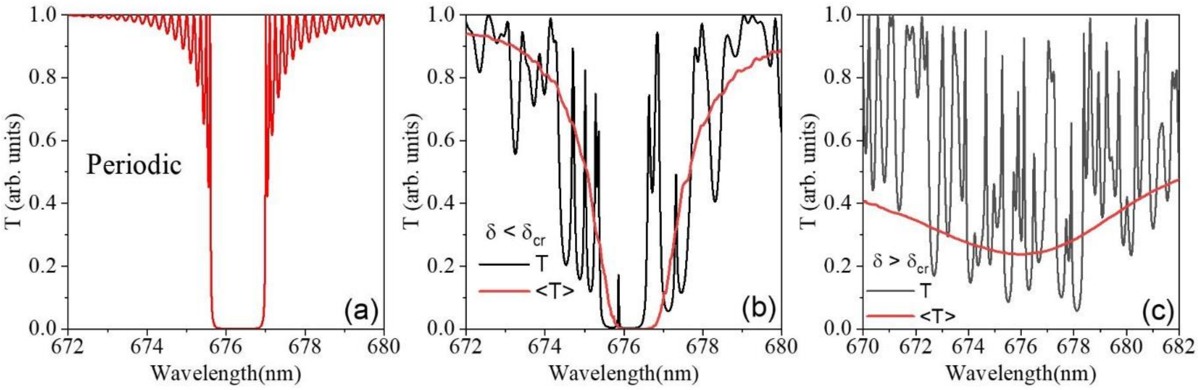


Fig. 2 (a) Computed transmission for a periodic structure. (b) At weak disorder ($\delta < \delta_{cr}$): Black curve shows transmission from a single configuration showing localized modes. Red curve: Configurationally-averaged transmission. (c) Same, at $\delta > \delta_{cr}$.

Figure 2 illustrates the realization of localized states in the spectra under disorder. Subplot (a) shows the periodic transmission spectrum. (b) depicts the single-configuration spectrum (red line) under

critical disorder ($\delta < \delta_{cr}$), showing localized modes formed in the gap, while the blue line shows the averaged spectrum over one thousand configurations. (c) depicts the same for $\delta > \delta_{cr}$. The estimation of critical disorder is made based on averaged transport <T>, since the Lifshitz tail is only defined for averaged transport. The experiment measures the averaged transport, whose spectra are then fit by the multiparameter fit described in the manuscript.

## III. Lifshitz-tail exponent and system size

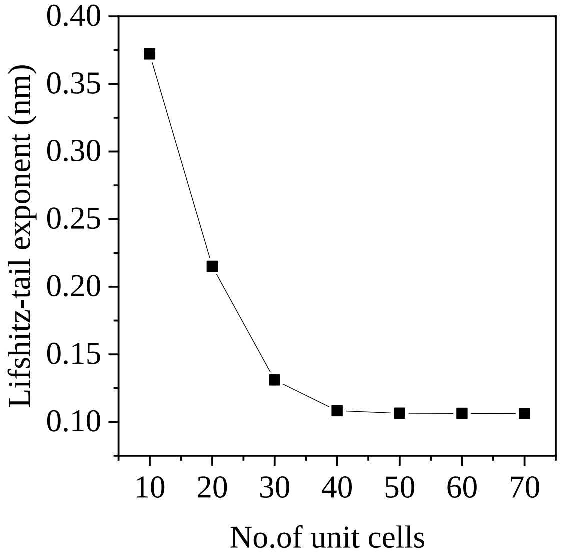


Fig. 3 Dependence of Lifshitz exponent on sample size. After about 40 unit cells, the size-dependence (originating from finite-size effects) is removed, and the exponent is independent of the size, and only depends on the strength of disorder.

Figure 3 shows the calculation of the Lifshitz exponent as a function of sample size. Upto about 40 unit cells, the Lifshitz tail is not fully evolved and hence finite-size effects are seen in the computation of the exponent. Thereafter, the sample is large enough and not affected by the size. The Lifshitz exponent is then independent of the sample size, and depends only on the strength of disorder.

## IV. Critical disorder

Critical disorder has been mainly discussed to manifest in two different ways, namely, in the statistics of transmission, and in the transition from multi-parameter scaling to single-parameter scaling. Here, we would like to show the agreement of our measured critical disorder with both these methods.

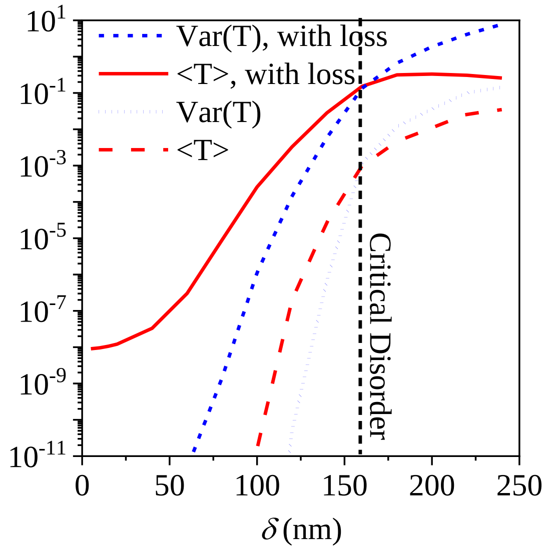


Fig.4 Dependence of mean and variance of transmittance at the mid gap at wavelength ~ 691.1 nm on disorder strength. Regardless of the loss, they cross at the critical disorder.

Kaliteevsky et al. show that a signature of criticality is the crossing of the profiles of mean and variance of transmittance (T) at the midgap as a function of disorder. Figure 4 in this document shows four traces. The mean transmittance (solid red trace) for a lossy system is seen to cross the variance of T (dashed blue line) at the mid gap at a disorder strength which matches the critical disorder given by Eqn. 1 (158 nm, dashed black vertical line). It is to be noted that the loss does not affect the critical disorder. The dashed red line and the dotted blue line show the mean and variance of transmittance in the same system made non-lossy. The crossing of the two curves is still at the same critical disorder, although the profiles are modified.

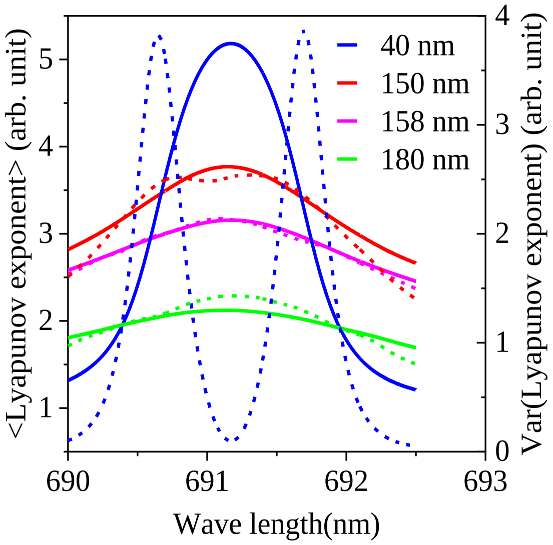


Fig. 4 Wavelength-dependence of mean (solid lines) and variance (dashed lines) of Lyapunov exponent in the region of the bandgap at ~ 691.1 nm, for different disorder strengths. The variance shows a dip at the midgap at weak disorder, which vanishes at the critical disorder after which the variance follows the mean. This coincides with the transition from multi-parameter scaling to one-parameter scaling.

Deych et al. discuss the failure of one-parameter scaling at very weak disorder. They study the wavelength dependence of mean and variance of Lyapunov exponent, defined as $\bar{\lambda} = -\frac{1}{L}\log(\mathrm{T})$. They show that the transition from a multi parameter scaling regime to a single parameter scaling occurs at the critical disorder. The critical disorder is identified using the variation in the functional dependence of mean and variance of the $\bar{\lambda}$. In a single parameter scaling regime, both variance and mean are governed by a single parameter unlike in a multi parameter scaling regime. Fig. 4 exhibits the statistics of the $\bar{\lambda}$ in our system. The solid lines indicate the mean of $\bar{\lambda}$, which shows a single peak at the midgap. The dashed lines show the var($\bar{\lambda}$), which has a dual-peaked profile at the disorder of 40 nm (blue lines) and 150 nm (red lines). At the critical disorder (158 nm), the variance also starts to show a single-peaked behaviour, indicating the transition into the single parameter scaling. This shows the equivalence of critical disorder in the two parameters, namely, <T> and $\bar{\lambda}$.
